# Supplementary material for: Direct observation of the band gap transition in atomically thin ReS$_2$
Source: arXiv:1702.04176 source file (2017-02-14)
Supplement: Supplementary file 1 [file SI.pdf]

# Supporting information: Direct observation of the band gap transition in atomically thin $ReS_2$

Mathias Gehlmann,[†] Irene Aguilera,[‡] Gustav Bihlmayer,[‡] Slavomír Nemšák,[†] Philipp Nagler,[¶] Pika Gospodarič,[†] Giovanni Zamborlini,[†] Markus Eschbach,[†] Vitaliy Feyer,[†] Florian Kronast,[§] Ewa Młyńczak,[†,‖] Tobias Korn,[¶] Lukasz Plucinski,[*,†] Christian Schüller,[¶] Stefan Blügel,[‡] and Claus M. Schneider[†]

*PGI-6, Forschungszentrum Jülich GmbH, Germany, PGI-1/IAS-1, Forschungszentrum Jülich GmbH and JARA, Germany, AG Schüller, University Regensburg, Germany, Abteilung Materialien für grüne Spintronik, Helmholtz-Zentrum Berlin, Germany, and Faculty of Physics and Applied Computer Science, AGH University of Science and Technology, Poland*

E-mail: l.plucinski@fz-juelich.de

## Band structure calculations

For our band structure calculations we used an angular momentum cutoff $l_{\max} = 8$ in the atomic spheres and a plane-wave cutoff of 4.0 bohr$^{-1}$ in the interstitial region. A $46 \times 46 \times 46$

[*]To whom correspondence should be addressed
[†]PGI-6, FZ-Jülich
[‡]PGI-1/IAS-1, FZ-Jülich
[¶]AG Schüller, University Regensburg
[§]Helmholtz-Zentrum Berlin
[‖]AGH University of Science and Technology

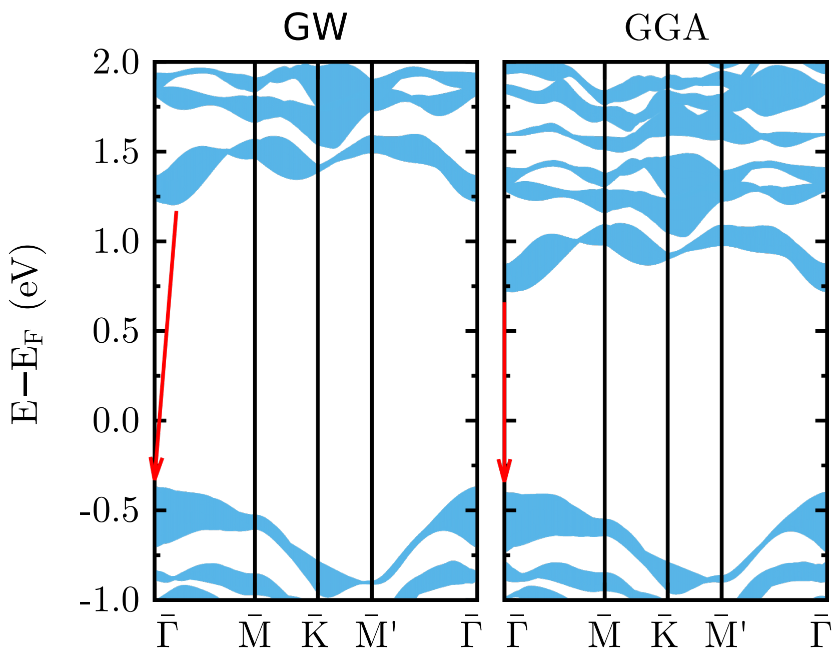


Figure 1: Comparison of bulk projected band structure calculated using GGA and GW.

k-point grid was used to sample the primitive BZ. For the *GW* calculations, a mixed product basis[1] was constructed with an angular momentum cutoff of $L_{\max} = 4$ and a plane-wave cutoff of 3.2 $\text{bohrs}^{-1}$. 520 unoccupied states and a $4{\times}4{\times}4$ k-point mesh were used in the *GW* calculations.

Figure 1 shows a direct comparison of our GGA and *GW* band structure calculations. The valence band structure is largely the same in both cases. However, the many-body effects, which are incorporated in *GW* lead to a significant increase of the band gap size and to an indirect band gap due to an altered conduction band dispersion.

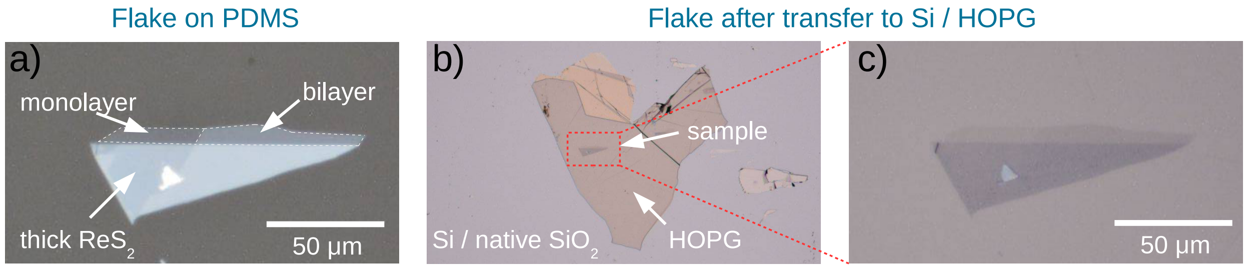


Figure 2: Optical microscope images of the atomically thin $ReS_2$ sample before (a) and after transfer (b-c) onto the substrate.

## References

(1) Friedrich, C.; Blügel, S.; Schindlmayr, A. *Phys. Rev. B* **2010**, *81*, 125102.
